# Supplementary material for: Observing interferences between past and future quantum states in resonance fluorescence
Source: arXiv:1311.5605 ancillary file (2014-05-15)
Supplement: Supplementary file 1 [file supmat.pdf]

# Supplementary information for "Observing interferences between past and future quantum states in resonance fluorescence"

P. Campagne-Ibarcq,[1,*] L. Bretheau,[1,*] E. Flurin,[1] A. Auffèves,[2] F. Mallet,[1] and B. Huard[1]

[1] *Laboratoire Pierre Aigrain, Ecole Normale Supérieure, CNRS (UMR 8551), Université P. et M. Curie, Université D. Diderot 24, rue Lhomond, 75231 Paris Cedex 05, France*

[2] *CNRS and Université Grenoble Alpes, Institut Néel, 38042 Grenoble, France*

## I. EXPERIMENTAL SETUP

The full experimental setup is presented on Fig. S1. The superconducting qubit follows the design of the "3D transmon" described in Ref. [1]. A single aluminum Josephson junction, connected to two antennas of 0.4 by 1mm each on a sapphire substrate, is embedded in an empty bulk aluminum cavity, anchored at base-temperature 20 mK of a dilution refrigerator. The transmon chip was fabricated by electron-beam lithography, double-angle evaporation, and oxidation to form the tunnel junction. Spectroscopic measurements give a qubit frequency $\nu_q = 5.19$ GHz that differs from the next transition by an anharmonicity $\alpha/2\pi = 160$ MHz. The measured relaxation time is $T_1 = 16$ $\mu$s, and the Ramsey time is $T_2 = 10.5$ $\mu$s.

Readout and drive pulses are generated by single side-band modulation of two continuous microwave tones produced by microwave generators set respectively at $\nu_{c0} + 62.5$ MHz and $\nu_q + 62.5$ MHz, where $\nu_{c0} = 7.74$ GHz is the cavity frequency at high power (Fig. S3.a). The modulation is performed by mixing these continuous waves with pulsed sinusoidal signals at 62.5 MHz synthesized by two different channels of a 4 channel Tektronix Arbitrary Waveform Generator. All sources are synchronized by an atomic clock. Both pulses are combined and sent towards the weakly coupled input port of the cavity through an input line which is filtered and attenuated with cryogenic attenuators at various stages of the dilution refrigerator, ensuring that negligible thermal excitations enter the device. A commercial (from K&L) low-pass clean-up filter of 12 GHz cut off frequency is used at the still stage (850 mK), while a home made low pass filter consisting in a microstrip line enclosed in an infrared tight box filled with Eccosorb is inserted at base temperature. Note that a similar line, denoted as "reflection probe" in Fig. S1, has been used for an in situ estimation of cavity input and output coupling rates $\Gamma_{a,b} = \frac{\gamma_{a,b}}{2\pi}$ (see section "Details of the model"), but is unused in the discussed experiment. Finally, the transmon aluminum 3D cavity is enclosed in an infrared tight copper box thermally anchored to the 20 mK stage. Its inside walls are all covered by a radiation absorbing coating consisting of 1 mm diameter SiC grains mixed up in Eccosorb.

Two cryogenic circulators in series are used to direct the outgoing fluorescence and readout signals from the cavity toward a Josephson mixer used as a low noise non degenerate amplifier at the qubit frequency $\nu_q$. A cryoperm magnetic shield encloses the Josephson mixer and its biasing coil (not shown). A third channel of the AWG is used to turn on ($\sim$ 30 dB of gain) or off (gain 1) the Josephson amplifier by DC-modulation of a continuous pump tone at 13.8 GHz. The output signal of the Josephson amplifier is then routed back towards a low noise HEMT (High Electron Mobility Transistor) amplifier of 40 dB gain from California Institute of Technology, isolated with a bias-tee and two circulators in series.

The output signal of the HEMT amplifier is further amplified at room temperature, then routed to a mixer driven, using a fast RF switch, either at $\nu_q + 62.5$ MHz when fluorescence is measured, or at $\nu_{c0} + 62.5$ MHz when the qubit state is finally readout (full representation of pulses scheme on Fig. S2). This scheme ensures that each of these two signals is mixed down to 62.5 MHz before being acquired by a 10-bit ADC at 2GS/s and numerically demodulated to extract both quadratures $V_{\mathrm{Re}}$ and $V_{\mathrm{Im}}$ using an FPGA board.

---

[*] These two authors contributed equally to this work

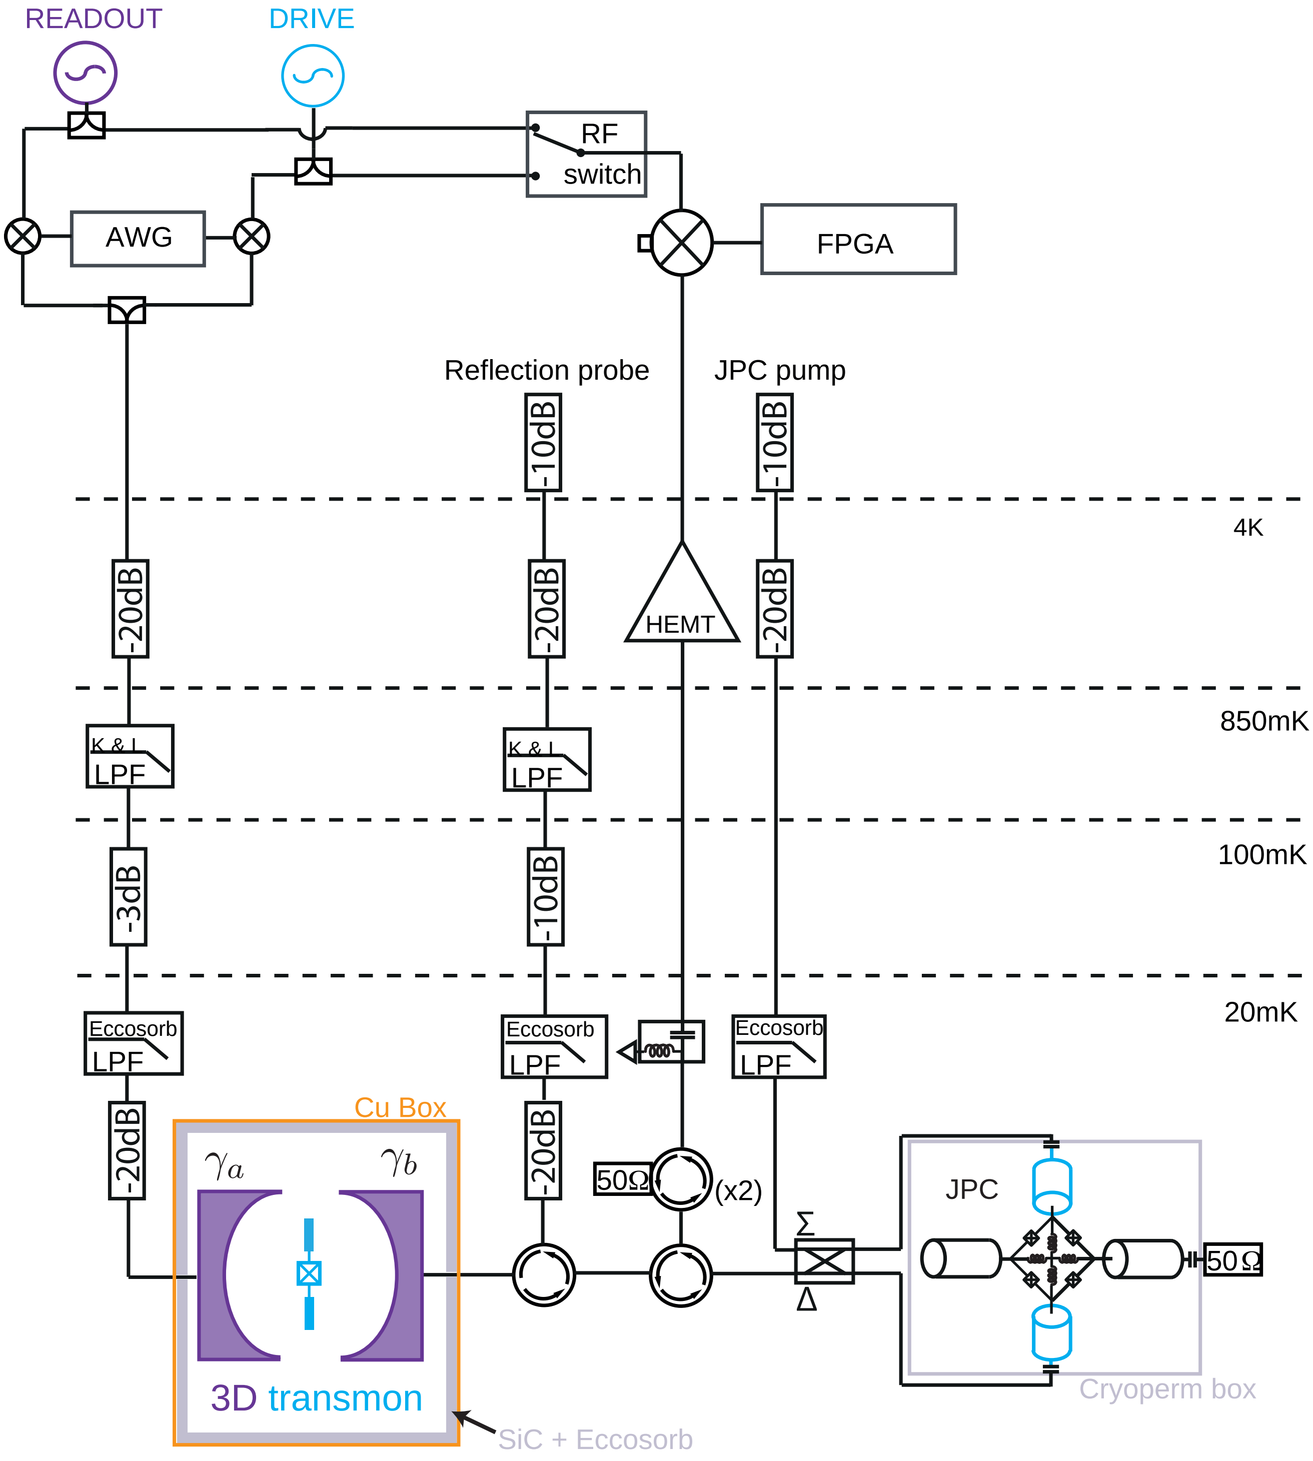


Figure S1: **Schematics of the experimental setup**

## II. PREPARATION AND MEASUREMENT FIDELITIES

### A. Preparation fidelity

In the absence of any active qubit cooldown scheme, thermal excitations in $|e\rangle$ would greatly limit the qubit's density matrix purity ($\sim$30% occupation of state $|e\rangle$), even before starting to drive the qubit. Then, higher excited

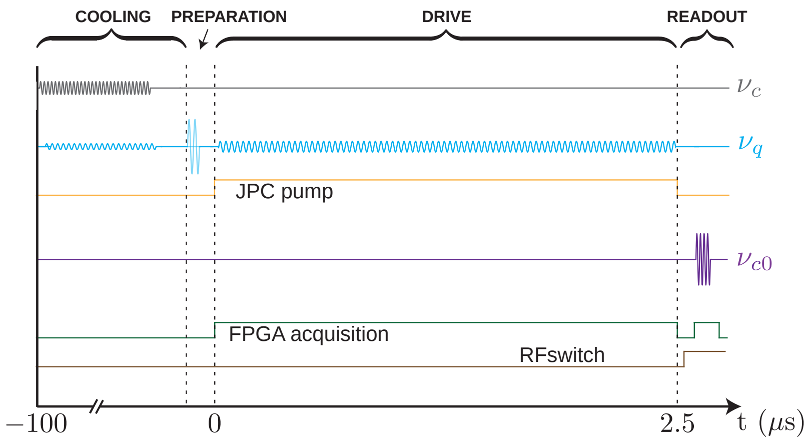


Figure S2: **Detailed pulse sequence**. All pulses are generated by modulating continuous microwave tones with waveforms generated by an Arbitrary Waveform Generator, synchronized with the clock of the acquisition board. The qubit is first cooled down for 100 $\mu$s using the method of Ref. [2]. After the end of these drives, a delay of 3 $\mu$s is used for intra cavity field to leak out. A fast $\pi$-pulse can then be applied for preparation of state $|e\rangle$. Qubit is then driven for 2.5 $\mu$s and the Josephson amplifier is turned on (pump on) in order to record fluorescence signal more efficiently. After the end of the drive, qubit state is readout using a high power pulse tuned at cavity bare frequency $\nu_{c0}$: for this purpose, the amplifier is turned off and the signal is down-converted at $\nu_{c0} + 62.5$ MHz, using a fast RF switch at room temperature.

states ($|f\rangle$ and above) would be occupied up to 9 % of the time, so that the approximation made by considering our transmon as a two-level system would not be accurate. We solve this problem by cooling down the qubit before every experiment using reservoir engineering as in Ref. [2]. When applying this cooling scheme long enough ( 100 $\mu$s $> T_1$), the occupation probability of the higher excited states is less than 1% at the beginning of every experiment reported in the letter.

The preparation efficiency is estimated by reading out the state of the qubit right after preparation in a separate experiment. Taking into account the finite readout fidelities described below, the $|e\rangle$ level remains excited only 9.5% of the time when preparing state $|g\rangle$, and gets as high as 84.6% when preparing state $|e\rangle$. This difference in purity is explained by two complementary effects. First, the relaxation of the qubit during the 500 ns of waiting time after the $\pi$-pulse preparing state $|e\rangle$. This waiting time was necessary in order to avoid polluting the fluorescence signal with the preparation pulse. Second, the $\pi$-pulse is inefficient when cavity photons remain after the cooling procedure, because the qubit frequency is shifted by $\chi_{cq}$ per photon, which makes the pulse out of resonance about 5 % of the time.

The maximally entropic state is described by a density matrix $\rho = (|g\rangle\langle g|+|e\rangle\langle e|)/2$. Given the preparation fidelities above, we can prepare $\rho_0 = 0.905|g\rangle\langle g| + 0.095|e\rangle\langle e|$ by cooling down the qubit and $\rho_1 = 0.154|g\rangle\langle g| + 0.846|e\rangle\langle e|$ by performing a $\pi$ pulse. In order to prepare $\rho = \mathbf{1}/2$, we work with a large ensemble of experiments in which 46.1% are prepared in $\rho_0$ and 53.9% in $\rho_1$. This is how we get an excellent preparation of the maximally entropic state despite not being able to prepare state $|e\rangle$ to better than 85%.

On a separate note, the relatively large temperature of the qubit at equilibrium does not reflect on the equilibrium occupation of the cavity mode. In fact, we can precisely determine the occupation of the cavity by looking at the spectroscopy of the qubit, since it exhibits peaks at $\nu_q - n\chi_{cq}$ for each integer $n$, whose amplitude reveals the probability to have $n$ photons. In practice, all peaks but the one corresponding to zero photons are below the noise floor of our measurement, which corresponds to an uncertainty of 4 % on the occupation of each level. Hence, at equilibrium, there are less than 0.04 average photons in the cavity. Note that the thermalization of the qubit and of the cavity are very different in nature since the qubit is quite thermally isolated on a sapphire chip poorly anchored inside of the superconducting cavity.

### B. Post-selection fidelity

In order to select sub-ensembles of experiments, one realizes a strong measurement of the qubit state at time $T$ using the high-power readout method [3]. Increasing the readout power above some threshold, the cavity resonance frequency switches to $\nu_{c0} = 7.74$ GHz. For a given pulse duration at $\nu_{c0}$ (here 200 ns), the threshold depends on qubit state, hence providing an efficient readout method. In practice, we found a maximal contrast between qubit states

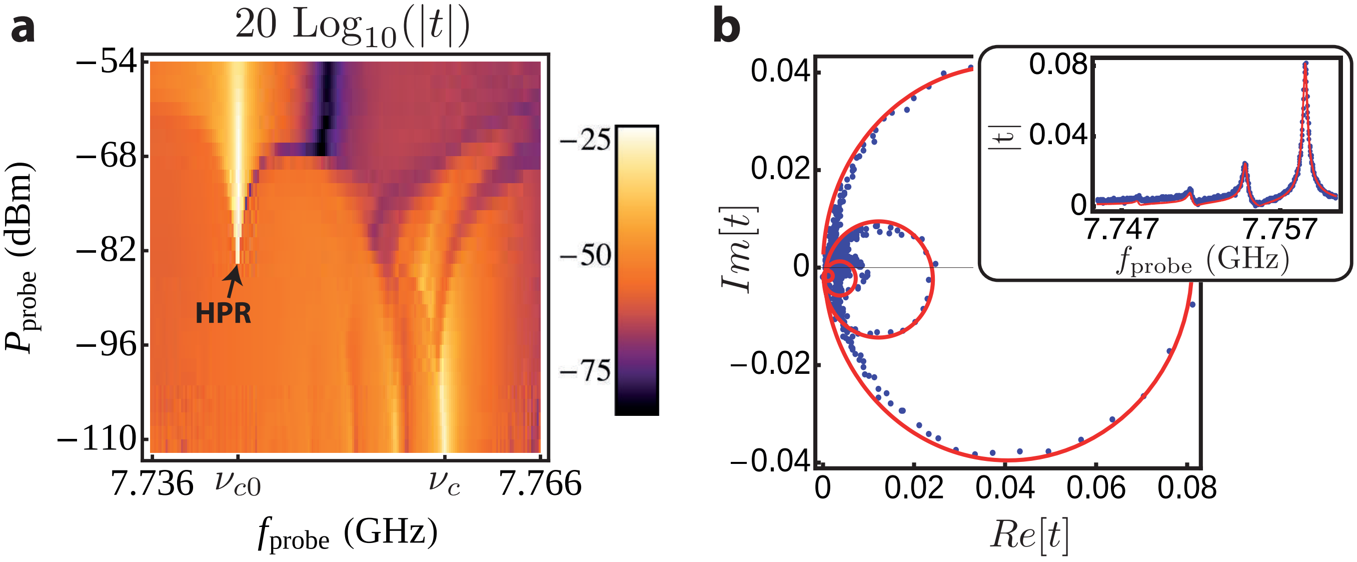


Figure S3: **a, High-power**. Transmission $t$ of the cavity (dB) encoded in color as a function of frequency and power at cavity input from the estimated attenuation on line $a$. Qubit is at thermal equilibrium before the measurement begins. Low-power resonance of the cavity (at $\nu_c$) is apparent on the bottom right part, with several replicas shifted by $-\chi$ (due to spurious thermal excitations of the qubit anharmonic oscillator). At high-power, cavity resonates at its bare frequency $\nu_{c0}$. High-power readout (HPR) is performed by sending a pulse in the region at the frontier between these two regimes, so that cavity response depends strongly on qubit state [3]. **b, Low-power.** Transmission of the cavity in the Fresnel plane (main panel) and in amplitude as a function of frequency (inset). The probing power is chosen such that there is $\sim 1$ photon on average inside cavity ( -152 dBm on Fig. a). The relative amplitudes of the resonances at $\nu_c$, $\nu_c - \chi$, $\nu_c - 2\chi$... reveal the thermal occupation of each level of the qubit: it is compatible with a Boltzman distribution at temperature $\sim 200$ mK (qubit excited with 29.5% probability).

for a power that would lead to about $1.5 \times 10^6$ photons on average in the cavity if the excitation were permanent.

The fidelities of the readout are defined by the conditional probabilities to observe switching $S$ (or no switching $\bar{S}$) events knowing the state of the qubit: $F_g = \mathcal{P}(\overline{\mathrm{S}}|g)$ and $F_e = \mathcal{P}(\mathrm{S}|e)$. We also define the unconditional probability $\mathcal{P}(S) = 1 - \mathcal{P}(\bar{S})$ to observe a switching event. In order to estimate these fidelities, we first need to extract independently the qubit thermal excitation probability. This is done by measuring the transmission of the cavity at low drive power with the qubit in thermal state. As shown on Fig. S3b, several resonance peaks are visible, corresponding to cavity shifts by various qubit states ($|g\rangle$, $|e\rangle$, $|f\rangle$...). By fitting the relative amplitudes of these peaks with a Boltzman distribution, one can access to the thermal occupation of the excited states. We find that excited qubit states are occupied up to 29.5% of the time at thermal equilibrium. Now to determine the fidelities, we compare the high power readout signal with or without a fast $\pi$-pulse inverting the occupations of states $|g\rangle$ and $|e\rangle$. Assuming a probability of switching for higher excited states of the qubit close to 1, we then extract the fidelities : $F_g \simeq F_e \simeq 96 \pm 1\%$.

Due to finite readout fidelity, the final measurement matrix $E$ has a purity smaller than 1, even at the final time T of the measurement. Quantitatively, and considering for example trajectories for which the final measurement indicates a qubit in $|g\rangle$, it reads: $E(T) = \mathcal{P}(g|\overline{\mathrm{S}})|g\rangle\langle g| + (1 - \mathcal{P}(g|\overline{\mathrm{S}}))|e\rangle\langle e|$. Neglecting the higher excited states ($|f\rangle$ and above) occupancy, a direct calculation leads to

$$\mathcal{P}(g|\overline{\mathrm{S}}) = \frac{F_g}{\mathcal{P}(\overline{S})} \frac{\mathcal{P}(\overline{S}) + F_e - 1}{F_g + F_e - 1}.$$

A symmetric formula can be derived for $\mathcal{P}(e|\mathrm{S})$, which will appear in the purity of $E(T)$ for qubit post selected in $|e\rangle$.

These conditional probabilities are very sensitive to readout fidelity, particularly when post-selecting trajectories that are rare. Theoretical predictions including the fidelities found above are in good agreement with experimental results overall. However, in some regions of time and Rabi frequency, the assumption of negligible occupation of state $|f\rangle$ leads to errors. In order to correct for this approximation, it is possible to artificially increase $F_e$. In practice, we have used $F_g = 96\%$ and $F_e = 99\%$ throughout the letter (see Figs. S4.a,b).

## III. DETAILS OF THE MODEL

### A. Adiabatic elimination of the cavity field operator

The qubit and cavity can be described by the Jaynes-Cumming Hamiltonian, valid in the rotative wave approximation:

$$\frac{H_{JC}}{h} = \nu_{q0}\frac{\sigma_z}{2} + \nu_{c0}\left(c^\dagger c + \frac{1}{2}\right) + \frac{g}{2\pi}\left(\sigma_+ c + \sigma_- c^\dagger\right). \tag{S1}$$

The first term is the qubit Hamiltonian, with $\nu_{q0}$ the qubit frequency not yet Lamb-shifted by the dressing of the cavity, and the Pauli matrices defined in the basis $\{|e\rangle, |g\rangle\}$ as

$$\begin{array}{c} \sigma_x = \begin{pmatrix} 0 & 1 \\ 1 & 0 \end{pmatrix},\ \sigma_y = \begin{pmatrix} 0 & -i \\ i & 0 \end{pmatrix},\ \sigma_z = \begin{pmatrix} 1 & 0 \\ 0 & -1 \end{pmatrix}, \\ \sigma_- = \begin{pmatrix} 0 & 0 \\ 1 & 0 \end{pmatrix},\ \sigma_+ = \begin{pmatrix} 0 & 1 \\ 0 & 0 \end{pmatrix},\ 1 = \begin{pmatrix} 1 & 0 \\ 0 & 1 \end{pmatrix} \end{array}. \tag{S2}$$

The second term describes the microwave cavity first mode and the final term represents a coupling of strength $g$ between the qubit mode and the cavity mode, which hybridizes the individual qubit and photon eigenstates.

In the input-output formalism, one can take into account finite coupling to transmission lines and qubit non radiative decay processes by considering the propagating modes[? ] $a_{in}$, $a_{out}$, $b_{in}$, $b_{out}$, $\xi_{in}$, $\xi_{out}$ verifying boundary conditions:

$$\begin{cases} a_{out} = \sqrt{\gamma_a}c - a_{in} \\ b_{out} = \sqrt{\gamma_b}c - b_{in} \\ \xi_{out} = \sqrt{\gamma_{nr}}\sigma_- - \xi_{in} \end{cases}, \tag{S3}$$

where $\gamma_b/2\pi = 0.25$ MHz is the coupling strength to line b, and $\gamma_a/2\pi = \gamma_L/2\pi \simeq 2$ kHz is the coupling strength to line a, approximately equal to the internal losses of the cavity $\gamma_L$. $\gamma_{nr}$ is the radiative decay rate of the qubit (spontaneous relaxation not due to the photonic part of the qubit excitation).

Then, in the Heisenberg picture, qubit and cavity follow the coupled Langevin equations of motion :

$$\begin{cases} \dot{c} = \frac{i}{\hbar}\left[H_{JC}, c\right] - \frac{\gamma_a+\gamma_b+\gamma_L}{2}c + \sqrt{\gamma_a}a_{in} + \sqrt{\gamma_b}b_{in} \\ \dot{\sigma_-} = \frac{i}{\hbar}\left[H_{JC}, \sigma_-\right] - \frac{\gamma_{nr}}{2}\sigma_- + \sqrt{\gamma_{nr}}\xi_{in} \end{cases}. \tag{S4}$$

In these equations, pure dephasing of the qubit has been neglected. Considering that $\Delta/2\pi = \nu_{c0} - \nu_{q0} \simeq 2.6$ GHz is the largest parameter of the system, in the frame rotating at $\nu_{q0}$, cavity reaches steady state nearly instantaneously at any time t so that one can perform the so-called adiabatic elimination of the cavity: $\dot{c} = 0$. Then, assuming that $\langle b_{in}\rangle = 0$ (no input drive via line b) and $\langle a_{in}\rangle = A$ is a semi-classical driving tone, one can show that:

$$\langle b_{out}\rangle = \langle b_{out}\rangle_0 - \sqrt{\gamma_{1b}}\langle\sigma_-\rangle. \tag{S5}$$

In the experiment, $\langle b_{out}\rangle_0$ is dominated by the direct parasitic leak between the lines $a$ and $b$. In the dispersive regime, $\gamma_{1b} = \gamma_b\frac{g^2}{\Delta^2}$ is the relaxation rate of the qubit through line b, which adds up to the non radiative decay rate to determine qubit's lifetime: $\gamma_1 \simeq \gamma_{nr} + \gamma_{1b}$. There are two ways of estimating the coupling factor $g$ leading to different results, hence to a different value of $\gamma_{1b}$.

- Through the shift of the cavity frequency once dressed by the qubit: from Eq (S4), one can show that $\nu_c - \nu_{c0} = \frac{g^2}{2\pi\Delta} \approx 16$ MHz (these two frequencies are shown on Fig. S3.a) so that $g/2\pi = 200$ MHz and one gets $\gamma_{1b} \simeq (102\ \mu\text{s})^{-1}$.
- Through the dispersive shift of the cavity when qubit goes from ground to excited state: this shift $\chi_{cq} = 2\alpha g^2/\Delta^2$ can be read directly on Fig. S3a and is $\chi_{cq}/2\pi = 3.8$ MHz. Recalling that the anharmonicity is $\alpha/2\pi = 160$ MHz, one finds $\gamma_{1b} \simeq (54\ \mu\text{s})^{-1}$.

These two values differ greatly and we believe that at least one of the models is wrong. Since the first method assumes that the high power limit of the cavity probe corresponds to the total absence of a qubit, whereas there are still antennas and a Josephson junction, it seems to us that it is the less reliable. However, we are not aware of any publication on this issue and prefer to show both results. Since the value of $\gamma_{1b}$ is simply informational in our experiment and has no impact on the rest of the letter, this is out of the scope of the present work.

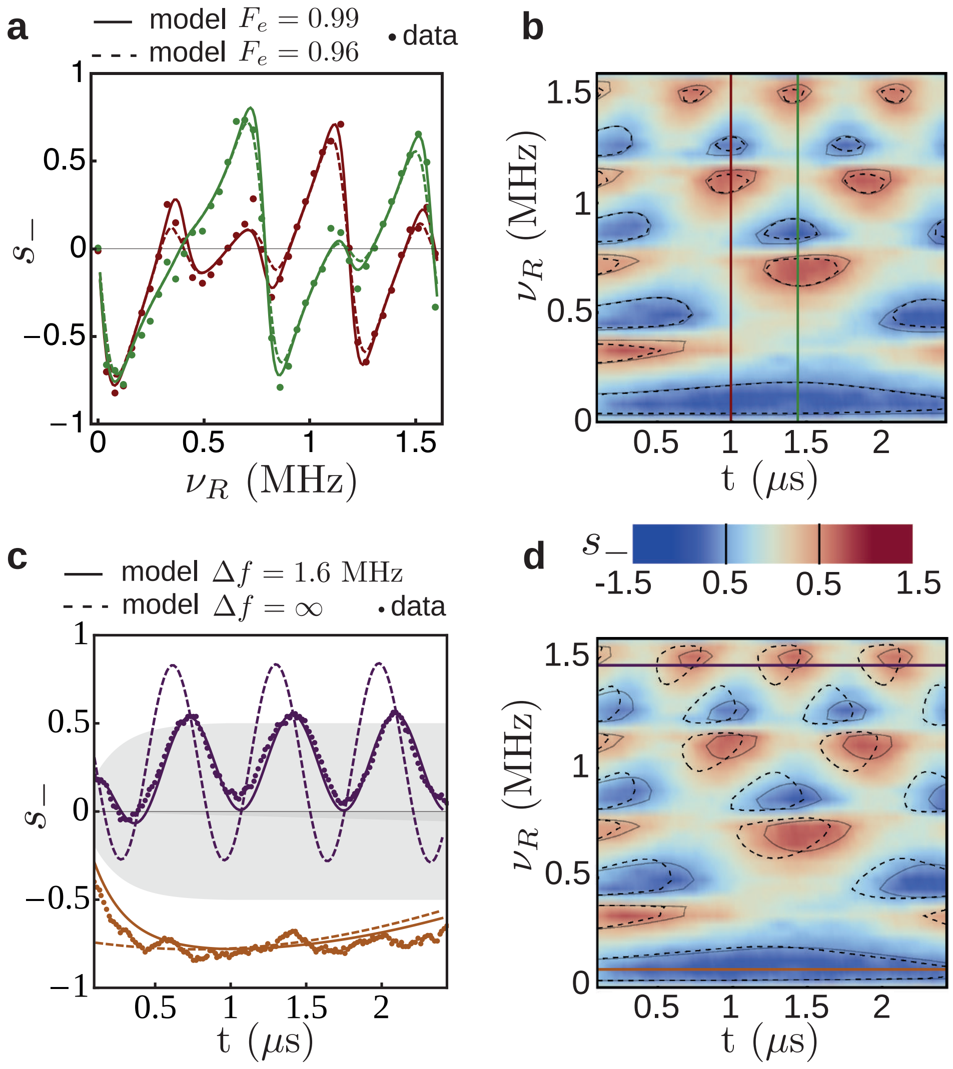


Figure S4: **a** Measured and expected conditional average fluorescence signals at $t = 0.99\ \mu$s (resp $t = 1.44\ \mu$s) are plotted in red (resp. green) as a function of Rabi frequency $\nu_R$ for a qubit prepared in $|e\rangle$ and post-selected in $|g\rangle$. Neglecting the higher excited qubit states leads to a small error on the postselection fidelity resulting in the dashed line ($F_g = F_e = 0.96$, dashed lines). Letting these fidelities be free parameters in order to account for these higher excited states allow for a slightly better agreement with the experiment at $F_g = 0.96$ and $F_g = 0.99$. **b** Same comparison for the whole set of data: measured $s_-$ is encoded in colour as a function of time $t$ and Rabi frequency $\nu_R$. Plain contours (resp. dashed contours) represent areas where the model with measured fidelities (resp. fitted fidelities) exceeds the classical range $[-0.5, 0.5]$. **c** For a qubit prepared in $|e\rangle$ and post-selected in $|g\rangle$, predicted fluorescence signal at frequencies $\nu_R = 0.08$ MHz (in brown) and $\nu_R = 1.47$ MHz (in purple) when considering a detection bandwidth of $\Delta f = 1.6$ MHz (plain lines) or with infinite bandwidth (dashed lines). Data (dots) are reasonably well reproduced by both models at low Rabi frequency compared to $\Delta f$, but not for higher frequency. The output of the finite bandwidth numerical filter to a square excitation of amplitude 0.5 delimits the gray region. The signal is considered to be beyond classical range only when trespassing this region, which is a conservative boundary. **d** Experimental fluorescence signal (in color) for the same preparation and post-selection conditions. Plain contours (resp. dashed contours) enclose regions of nonclassical values for $\Delta f = 1.6$ MHz (resp. infinite). The finite bandwidth introduce both a delay and some attenuation, especially at large $\nu_R$. The purple and orange lines correspond to the dots in c).

### B. Measurement Strength

As described above, the fluorescence signal is a propagating signal whose amplitude is of the order of $\sqrt{\gamma_{1b}}$. That means that the average number of photons in the signal per unit of time is $\gamma_{1b}$. The detector has a bandwidth $\Delta f = 1.6$ MHz limited by the Josephson amplifier of power gain $G = 10^3$. The average number of signal photons in the amplifier resonator is thus of the order of $G\gamma_{1b}/\Delta f \approx 6$. The quantum noise level in the amplifier resonator corresponds to $G - 1/2 \approx G$ average photons. Therefore, the measurement strength, which is the signal to noise

ratio [4], is of the order of $\gamma_{1b}/\Delta f \approx 0.1$ %. This number corresponds to the measurement strength of the shortest independent measurement time, which is $1/\Delta f$. If the measurement lasts for a time $T_m > 1/\Delta f$, the measurement strength is $\gamma_{1b}T_m$ as long as this number is much smaller than 1. In our experiment, even if one would consider the whole recording of fluorescence from $t = 0$ to $t = T$, the measurement performed by the fluorescence is weak since $\gamma_{1b}T \lesssim 3$ %.

### C. Taking into account detector bandwidth in the time domain

The predictions of the average values (conditional or not) of $\sigma_-$ are expected to reproduce the fluorescence signal $s_-^{(\mathrm{ideal})}(t)$ one would measure with a perfect detector. In practice, the detection setup has a bandwidth of 1.6 MHz which distorts the signal and needs to be modeled in order to compare theory and experiment. Starting from a predicted $s_-^{(\mathrm{ideal})}(t)$, we use a numerical filter corresponding in Fourier domain to a Lorentzian shape transmission centered at $\nu_q$ and with full width at half maximum $\Delta f = 1.6$ MHz. The deformation can be observed in Figs. S4c and S4d where both the unfiltered and the filtered signals are represented.

Apart from that treatment, a global scaling factor, used for all the measured data in the letter, is used to take into account the gain of the detection setup. The figure we find is consistent with the detection setup.

In Fig. 3 of the letter, the contours delimiting the classical boundaries also take into account the finite bandwidth of the detector. Ideally, they should reflect the regions of time $t$ and Rabi frequency $\nu_R$ where $|s_-^{(\mathrm{ideal})}(t)| > 0.5$. In practice, in order to avoid complex post-treatment of the data, we calculated the output of the detection setup for a square signal going instantaneously from 0 to 0.5: $s_-^{(\mathrm{ideal})}(t) = 0.5\Theta(t)$. This leads to a conservative estimation of the regions where macro-realism is violated.

## IV. COMPLEMENTARY EXPERIMENTAL RESULTS

Measured and predicted fluorescence signals for every preparation and post-selection conditions we have investigated are represented on Fig. S5. Signal value is encoded in color as a function of time $t$ and Rabi frequency $\nu_R$. Regions in which signal goes beyond classical range are enclosed in black contours. When $\pi\nu_R T$ is an integer number, the past and future knowledge either maximally agree or maximally disagree. In the latter case, $\tilde{\rho} = 0$ and $\langle\sigma_-\rangle_w$ is zero. This happens for odd numbers of $\pi$ rotations for $|e\rangle$ to $|e\rangle$ and $|g\rangle$ to $|g\rangle$ and even numbers for $|e\rangle$ to $|g\rangle$ and $|g\rangle$ to $|e\rangle$.

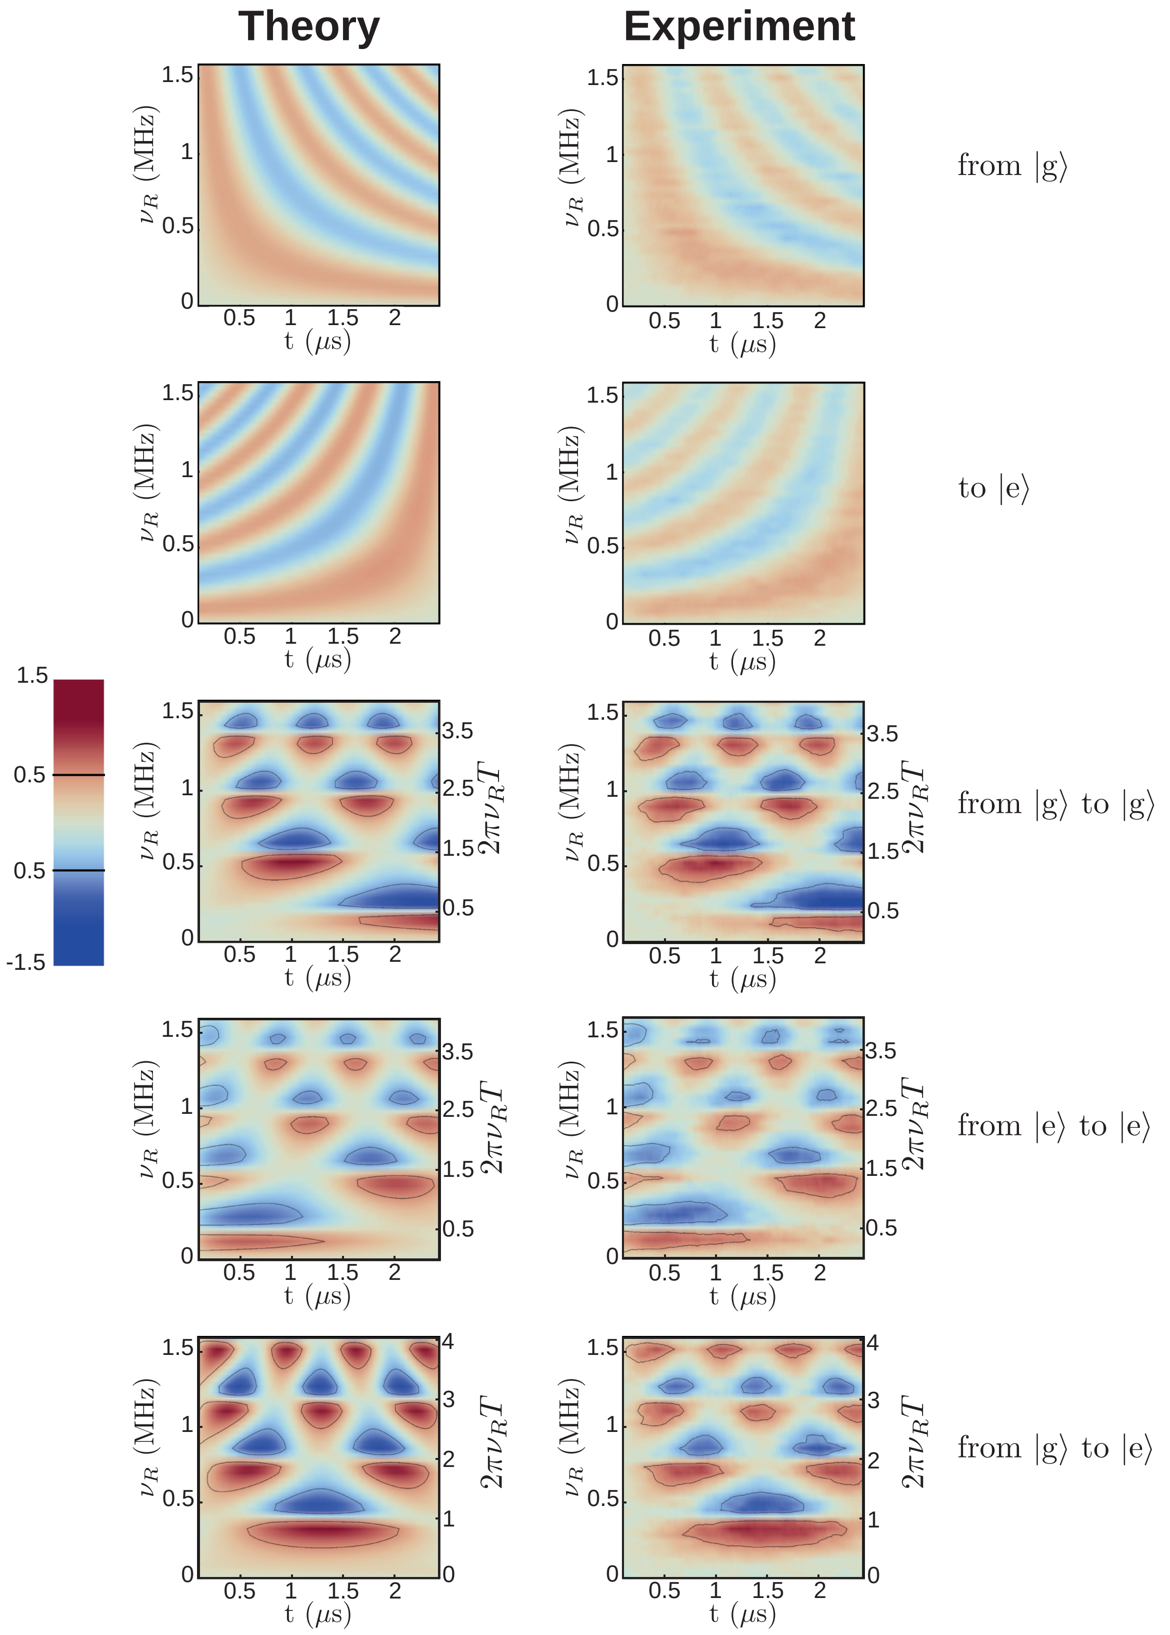


Figure S5: **Comparison between experiment and theory**

[1] Paik, D. Schuster, Bishop, G. Kirchmair, G. Catelani, Sears, Johnson, Reagor, Frunzio, Glazman, Girvin, Devoret and Schoelkopf. Observation of High Coherence in Josephson Junction Qubits Measured in a Three-Dimensional Circuit QED Architecture. *Physical Review Letters* **107**, 240501 (2011).

[2] K. Geerlings, Z. Leghtas, I. M. Pop, S. Shankar, L. Frunzio, R. J. Schoelkopf, M. Mirrahimi and M. H. Devoret. Demonstrating a Driven Reset Protocol for a Superconducting Qubit. *Physical Review Letters* **110**, 120501 (2013).

[3] M. D. Reed, L. DiCarlo, B. R. Johnson, L. Sun, D. I. Schuster, L. Frunzio and R. J. Schoelkopf. High-Fidelity Readout in Circuit Quantum Electrodynamics Using the Jaynes-Cummings Nonlinearity. *Physical Review Letters* **105**, 173601 (2010).

[4] A. A. Clerk, M. H. Devoret, S. M. Girvin, F. Marquardt and R. J. Schoelkopf. Introduction to quantum noise, measurement, and amplification. *Reviews of Modern Physics* **82**, 1155–1208 (2010).

[5] $a_{in}$ and $a_{out}$ (resp. $b_{in}$ and $b_{out}$) are the propagating modes of line $a$ (resp. $b$) going towards and outwards the cavity. Modes $\xi_{in}$ and $\xi_{out}$ model the input/output modes of the qubit relaxation channel that is not due to the coupling to lines $a$ and $b$.
